# Supplementary material for: DStruct2Design: Data and Benchmarks for Data Structure Driven Generative Floor Plan Design
Source: arXiv:2407.15723 source file (2024-07-22)
Supplement: Supplementary file 1 [file Supplementary.tex]

\appendix

\section{Dataset Datasheet}

\subsection{Motivation}

\subsubsection{For what purpose was the dataset created? (Was there a specific task in mind? Was there a specific gap that needed to be filled? Please provide a description.)}
The dataset was created to address the need for floorplan generation that adheres to numerical constraints, such as room sizes, which are crucial for practical applications. It fills a gap in current approaches and datasets that do not support these kinds of constraints. 

\subsubsection{Who created this dataset (e.g., which team, research group), and on behalf of which entity (e.g., company, institution, organization)?}
It was created at Mila - Quebec Artificial Intelligence Institute, in Chris Pal’s research group by Zhi Hao Luo and Luis Lara.

\subsubsection{Who funded the creation of the dataset? (If there is an associated grant, please provide the name of the grantor and the grant name and number.)}
The dataset was funded by Mila and CIFAR.

\subsubsection{Any other comments?}
None.

\subsection{Composition}

\subsubsection{What do the instances that comprise the dataset represent (e.g., documents, photos, people, countries)? Are there multiple types of instances (e.g., movies, users, and ratings; people and interactions between them; nodes and edges)? Please provide a description.} 
An instance of the dataset contains details about the layout and specifications of a building or a floor plan. Specifically, each instance includes the following elements: the total number of rooms ("room\_count"), the total area in square units ("total\_area"), and a list of room types present ("room\_types"). Additionally, it contains a list of individual room dictionaries ("rooms"), where each dictionary details specific room characteristics such as the area of the room ("area"), a list of vertices defining the room's layout ("floor\_polygon") with coordinates ("x" and "y"), and a flag indicating if the room's shape is rectangular ("is\_regular"). Each room also includes the dimensions of its bounding box ("height" and "width"), a unique identifier ("id"), the type of the room ("room\_type"), and a list of edges ("edges"). 

\subsubsection{How many instances are there in total (of each type, if appropriate)?}
In total, there are 92,315 instances of house layouts. ProcTHOR-10k contributes with 12,000 because we included training, validation, and test instances. Meanwhile, RPLAN offers a dataset with 80,315 instances. 

\subsubsection{Does the dataset contain all possible instances or is it a sample (not necessarily random) of instances from a larger set? If the dataset is a sample, then what is the larger set? Is the sample representative of the larger set (e.g., geographic coverage)? If so, please describe how this representativeness was validated/verified. If it is not representative of the larger set, please describe why not (e.g., to cover a more diverse range of instances, because instances were withheld or unavailable).}
Our dataset is not a sample from a larger dataset. It is a complete and unique combination of the ProcTHOR-10k and RPLAN datasets.

\subsubsection{What data does each instance consist of? “Raw” data (e.g., unprocessed text or images) or features? In either case, please provide a description.}
Each instance in the ProcTHOR-10K dataset consists of a raw, procedurally generated 3D house. For RPLAN, each instance consists of raw 256 × 256 × 4 vector images representing real-world floor plans from Asia, where each channel contains specific boundary and room information. 

\subsubsection{Is there a label or target associated with each instance? If so, please provide a description.}
While no explicit label or target is associated with each instance of the dataset, several attributes of each instance can be used as targets. For instance, we used different target settings in our experiments.

\subsubsection{Is any information missing from individual instances?  If so, please provide a description, explaining why this information is missing (e.g., because it was unavailable). This does not include intentionally removed information, but might include, e.g., redacted text.}
There is no missing information.

\subsubsection{Are relationships between individual instances made explicit (e.g., users’ movie ratings, social network links)? If so, please describe how these relationships are made explicit.}
No, each instance in the dataset is treated independently, focusing on generating and evaluating individual floor plans. Each floor plan is generated based on its own set of constraints and characteristics, without any reference to or relationship with other instances.

\subsubsection{Are there recommended data splits (e.g., training, development/validation, testing)? If so, please provide a description of these splits, explaining the rationale behind them.}
No, we do not recommend specific data splits. In our experiments,  we use random splits as described in our paper.

\subsubsection{Are there any errors, sources of noise, or redundancies in the dataset? If so, please provide a description.}
No but the following processes inherently risk introducing errors and noise into the dataset. Firstly, converting existing image-based floorplan and 3D house datasets (RPLAN and ProcTHOR-10K) into JSON-based data structures may introduce errors or inconsistencies, particularly in accurately defining room boundaries and vertices. Secondly, the cleaning process removes redundant points and applies rounding to coordinates for consistency. Finally, manual annotation in datasets like RPLAN could be a source of noise due to human errors in labeling and tracing room perimeters.  

\subsubsection{Is the dataset self-contained, or does it link to or otherwise rely on external resources (e.g., websites, tweets, other datasets)? If it links to or relies on external resources, a) are there guarantees that they will exist, and remain constant, over time; b) are there official archival versions of the complete dataset (i.e., including the external resources as they existed at the time the dataset was created); c) are there any restrictions (e.g., licenses, fees) associated with any of the external resources that might apply to a dataset consumer? Please provide descriptions of all external resources and any restrictions associated with them, as well as links or other access points, as appropriate.}
The dataset relies on external resources, and there are potential issues with the availability and consistency of these resources over time. 

\begin{enumerate}[label=(\alph*)]
\item There are no guarantees that these external resources will exist and remain constant over time. 
\item No, the complete dataset has no official archival version. However, a partial version of our dataset, specifically the ProcTHOR-10K portion, is saved on HuggingFace.
\item There are restrictions associated with the RPLAN dataset. The RPLAN dataset involves real-world floor plans that have usage restrictions, including licenses that prevent redistribution or require permission for use. Users must adhere to these licensing terms, which may limit how the data can be shared or utilized in subsequent projects. The following is the link to the 
\href{https://drive.google.com/file/d/1wEbccL5NAL\_mzFt2hyxPqZppXDalbApW/view}{RPLAN Terms of Use }.
\end{enumerate}

\subsubsection{Does the dataset contain data that might be considered confidential (e.g., data that is protected by legal privilege or by doctor– patient confidentiality, data that includes the content of individuals’ non-public communications)? If so, please provide a description.}
The RPLAN dataset is created using anonymized floorplan data, ensuring no user or privacy information is included, thus eliminating potential confidentiality concerns. Additionally, the ProcTHOR-10K dataset is procedurally generated, further ensuring the absence of sensitive information. Therefore, our dataset does not contain any data that might be considered confidential, such as information protected by legal privilege or doctor-patient confidentiality, or content from individuals’ non-public communications.

\subsubsection{Does the dataset contain data that, if viewed directly, might be offensive, insulting, threatening, or might otherwise cause anxiety? If so, please describe why. If the dataset does not relate to people, you may skip the remaining questions in this section.}
No.

\subsubsection{Does the dataset identify any subpopulations (e.g., by age, gender)? If so, please describe how these subpopulations are identified and provide a description of their respective distributions within the dataset.}
No.

\subsubsection{Is it possible to identify individuals (i.e., one or more natural persons), either directly or indirectly (i.e., in combination with other data) from the dataset? If so, please describe how.}
No, it is not possible to identify individuals, either directly or indirectly, from the dataset. 

\subsubsection{Does the dataset contain data that might be considered sensitive in any way (e.g., data that reveals race or ethnic origins, sexual orientations, religious beliefs, political opinions or union memberships, or locations; financial or health data; biometric or genetic data; forms of government identification, such as social security numbers; criminal history)? If so, please provide a description.}
No.

\subsubsection{Any other comments?}
None.

\subsection{Collection Process}

\subsubsection{How was the data associated with each instance acquired? Was the data directly observable (e.g., raw text, movie ratings), reported by subjects (e.g., survey responses), or indirectly inferred/derived from other data (e.g., part-of-speech tags, model-based guesses for age or language)? If the data was reported by subjects or indirectly inferred/derived from other data, was the data validated/verified? If so, please describe how.}
The data associated with each instance was indirectly inferred and derived from other data sources. There are no specific validation or verification steps for the derived data beyond the preprocessing and cleaning procedures described.

\subsubsection{What mechanisms or procedures were used to collect the data (e.g., hardware apparatuses or sensors, manual human curation, software programs, software APIs)? How were these mechanisms or procedures validated?}
The data was collected through a combination of manual human curation and software programs. The RPLAN dataset involved manual annotation and extraction of floorplans from real-world sources, ensuring detailed and accurate data. The ProcTHOR dataset was procedurally generated using simulation software designed to create interactive 3D house layouts. We used software programs to convert these datasets into a JSON-based data structure. No extra validation mechanisms were conducted.

\subsubsection{If the dataset is a sample from a larger set, what was the sampling strategy (e.g., deterministic, probabilistic with specific sampling probabilities)?}
The dataset is not a sample from a larger set.

\subsubsection{Who was involved in the data collection process (e.g., students, crowdworkers, contractors) and how were they compensated (e.g., how much were crowdworkers paid)?}
The authors carried out the data collection process. No crowd workers, contractors, or external personnel were involved in this process.

\subsubsection{Over what timeframe was the data collected? Does this timeframe match the creation timeframe of the data associated with the instances (e.g., recent crawl of old news articles)? If not, please describe the timeframe in which the data associated with the instances was created.}
The data was collected over the span of a week. This timeframe does not match the creation timeframe of the data associated with the instances, as the original RPLAN and ProcTHOR datasets were created earlier and over a longer period.

\subsubsection{Were any ethical review processes conducted (e.g., by an institutional review board)? If so, please provide a description of these review processes, including the outcomes, as well as a link or other access point to any supporting documentation. If the dataset does not relate to people, you may skip the remaining questions in this section.}
No.

\subsubsection{Did you collect the data from the individuals in question directly, or obtain it via third parties or other sources (e.g., websites)?}
We did not collect the data from individuals directly. Instead, we obtained the data via third parties or other sources, specifically from the RPLAN and ProcTHOR datasets.

\subsubsection{Were the individuals in question notified about the data collection? If so, please describe (or show with screenshots or other information) how notice was provided, and provide a link or other access point to, or otherwise reproduce, the exact language of the notification itself.}
The individuals in question were not directly notified about the data collection, but we are following their research project terms of use and licenses.

\subsubsection{Did the individuals in question consent to the collection and use of their data? If so, please describe (or show with screenshots or other information) how consent was requested and provided, and provide a link or other access point to, or otherwise reproduce, the exact language to which the individuals consented.}
For the RPLAN dataset, we followed the RPLAN Terms of Use and filled out the corresponding form. Besides, we adhered to the ProcTHOR-10K dataset's Apache License, which governs its use and distribution. Both datasets were obtained and used in compliance with their respective terms, ensuring proper and ethical data-handling practices.

\subsubsection{If consent was obtained, were the consenting individuals provided with a mechanism to revoke their consent in the future or for certain uses? If so, please provide a description, as well as a link or other access point to the mechanism (if appropriate).}
They did not provide a mechanism to revoke their consent. 

\subsubsection{Has an analysis of the potential impact of the dataset and its use on data subjects (e.g., a data protection impact analysis) been conducted? If so, please provide a description of this analysis, including the outcomes, as well as a link or other access point to any supporting documentation.}
No.

\subsubsection{Any other comments?}
None.

\subsection{Preprocessing/cleaning/labeling}

\subsubsection{Was any preprocessing/cleaning/labeling of the data done (e.g., discretization or bucketing, tokenization, part-of-speech tagging, SIFT feature extraction, removal of instances, processing of missing values)? If so, please provide a description. If not, you may skip the remaining questions in this section.}
Yes, preprocessing and cleaning of the data were conducted for both ProcTHOR-10k and RPLAN datasets. For ProcTHOR-10k, the raw data from each house was processed with a focus on the geometric properties of the rooms. This involved using the shoelace formula to calculate areas and determining room dimensions based on their x and y coordinates. Redundant points were removed, and coordinates were rounded for consistency. Additionally, rooms were categorized and counted by type, and the total area for each house layout was computed. For the RPLAN dataset, the 4-channel vector images were converted into a JSON structure. This process included extracting all pixel coordinates for each room, tracing the room perimeters to capture vertices in order, and deducing room types along with other relevant fields.

\subsubsection{Was the “raw” data saved in addition to the preprocessed/cleaned/labeled data (e.g., to support unanticipated future uses)? If so, please provide a link or other access point to the “raw” data.}
The raw data came directly from their authors and can be accessed through the provided links: \href{https://github.com/allenai/procthor-10k}{ProcTHOR-10k} and \href{http://staff.ustc.edu.cn/~fuxm/projects/DeepLayout/}{RPLAN}.

\subsubsection{Is the software that was used to preprocess/clean/label the data available? If so, please provide a link or other access point.}
The preprocess and cleaning code is available at https://github.com/plstory/DS2D

\subsubsection{Any other comments?}
None.

\subsection{Uses}

\subsubsection{Has the dataset been used for any tasks already? If so, please provide a description.}
Yes, we used to train the model called DStruct2Design (DS2D) LLM that we presented in the paper.

\subsubsection{Is there a repository that links to any or all papers or systems that use the dataset? If so, please provide a link or other access point.}
Our repository project is https://github.com/plstory/DS2D

\subsubsection{What (other) tasks could the dataset be used for?}
It could aid in architectural design and planning by helping architects generate and modify floorplans that meet specific numerical criteria, such as room sizes and spatial arrangements. Interior designers could optimize furniture and fixture placement within specified room dimensions, ensuring efficient use of space. Additionally, game developers could utilize the dataset to create dynamic and customizable in-game environments, ensuring that generated spaces meet specific design criteria and enhance gameplay. 

\subsubsection{Is there anything about the composition of the dataset or the way it was collected and preprocessed/cleaned/labeled that might impact future uses? For example, is there anything that a dataset consumer might need to know to avoid uses that could result in unfair treatment of individuals or groups (e.g., stereotyping, quality of service issues) or other risks or harms (e.g., legal risks, financial harms)? If so, please provide a description. Is there anything a dataset consumer could do to mitigate these risks or harms?}
No.

\subsubsection{Are there tasks for which the dataset should not be used? If so, please provide a description.}
No tasks come to our mind for which the dataset should not be used.

\subsubsection{Any other comments?}
None.

\subsection{Distribution}

\subsubsection{Will the dataset be distributed to third parties outside of the entity (e.g., company, institution, organization) on behalf of which the dataset was created? If so, please provide a description.}
Yes, we will use Hugging Face as the platform for distribution a partial version of our dataset, specifically the ProcTHOR-10K portion. 

\subsubsection{How will the dataset will be distributed (e.g., tarball on website, API, GitHub)? Does the dataset have a digital object identifier (DOI)?}
Via Hugging Face datasets for distribution a partial version of our dataset, specifically the ProcTHOR-10K portion. 

\subsubsection{When will the dataset be distributed?}
It will be distributed in the 2024 summer. 

\subsubsection{Will the dataset be distributed under a copyright or other intellectual property (IP) license, and/or under applicable terms of use (ToU)? If so, please describe this license and/or ToU, and provide a link or other access point to, or otherwise reproduce, any relevant licensing terms or ToU, as well as any fees associated with these restrictions.}
We used the Apache-2.0 license for our code and for the partial version of our dataset, which included only the ProcTHOR-10k part and was saved in Hugging Face.

\subsubsection{Have any third parties imposed IP-based or other restrictions on the data associated with the instances? If so, please describe these restrictions, and provide a link or other access point to, or otherwise reproduce, any relevant licensing terms, as well as any fees associated with these restrictions.}
The ProcTHOR-10k dataset is available under the Apache License 2.0, distributed with the Allen Institute for AI’s prior package, indicating no significant third-party restrictions. Contrarily, the redistribution of the RPLAN data is prohibited, meaning that our new dataset derived from RPLAN cannot be directly shared. Instead, researchers must download the RPLAN dataset from the source and use the provided code to recreate the dataset, complying with the redistribution restrictions.

\subsubsection{Do any export controls or other regulatory restrictions apply to the dataset or to individual instances? If so, please describe these restrictions, and provide a link or other access point to, or otherwise reproduce, any supporting documentation.}
Yes, for RPLAN, refer to their Terms of Use, and for ProcTHOR-10k, the applicable license is the Apache License.

\subsubsection{Any other comments?}
None.

\subsection{Maintenance}

\subsubsection{Who will be supporting/hosting/maintaining the dataset?} 
Luis Lara.

\subsubsection{How can the owner/curator/manager of the dataset be contacted (e.g., email address)?} 
luis.lara@mila.quebec

\subsubsection{Is there an erratum? If so, please provide a link or other access point.}
No.

\subsubsection{Will the dataset be updated (e.g., to correct labeling errors, add new instances, delete instances)? If so, please describe how often, by whom, and how updates will be communicated to dataset consumers (e.g., mailing list, GitHub)?}
No plans to update it yet but open to doing it if necessary. 

\subsubsection{If the dataset relates to people, are there applicable limits on the retention of the data associated with the instances (e.g., were the individuals in question told that their data would be retained for a fixed period of time and then deleted)? If so, please describe these limits and explain how they will be enforced.}
No.

\subsubsection{Will older versions of the dataset continue to be supported/hosted/maintained? If so, please describe how. If not, please describe how its obsolescence will be communicated to dataset consumers.}
No.

\subsubsection{If others want to extend/augment/build on/contribute to the dataset, is there a mechanism for them to do so? If so, please provide a description. Will these contributions be validated/verified? If so, please describe how. If not, why not? Is there a process for communicating/distributing these contributions to dataset consumers? If so, please provide a description.}
Contributors are encouraged to create a Pull Request (PR) in the project's GitHub repository. Once a PR is submitted, the contributions will be validated and verified through a review process. Approved changes will be merged into the repository's main branch and documented in the project's changelog or release notes. The above ensures that all dataset users are informed about the updates and can access the latest version.

\subsubsection{Any other comments?}
None.

\section{URL to Croissant Record}
Our Croissant metadata record can be found here:

\textbf{https://huggingface.co/datasets/ludolara/DStruct2Design}

\section{Author Statement}
We the authors bear responsibility in case of violation of rights in using this data. We follow the Apache 2.0 License declared by ProcTHOR. For RPLAN, we strictly adhere to the creator's request for it to be only obtained through request from its source, and for it to be non-commercial research and academic purposes. We do not distribute RPLAN in any way; we provide a conversion tool to be used on RPLAN.

\section{Hosting, Licensing, Maintenance}

\subsection{Hosting}
GitHub hosts the code to train our model, run the benchmark, and create the dataset. Hugging Face hosts a subset version of our dataset, which included only the ProcTHOR-10k. However, the user must follow the repository's instructions to generate the complete dataset that includes ProcTHOR-10k and RPLAN.

\subsection{Licensing}
We used the Apache-2.0 license for our code and for the partial version of our dataset, which included only the \textbf{ProcTHOR-10k}. We cannot share our new dataset directly due to the redistribution restrictions of the \textbf{RPLAN} described in their terms of use. However, after downloading the \textbf{RPLAN} from the author's source, the code provided in the repository can be used to fully create our dataset.

\subsection{Maintenance}

This repository will also be actively maintained and updated by the authors for better code readability and ease of use. We will also update instructions in the Readme file accordingly, e.g., when datasets are hosted in a different place, for better accessibility. We will continuously update the repository to ensure it is easy to reproduce our results.

Contributors are encouraged to create a Pull Request (PR) in the project's GitHub repository. Once a PR is submitted, the contributions will be validated and verified through a review process. Approved changes will be merged into the repository's main branch and documented in the project's changelog or release notes. The above ensures that all dataset users are informed about the updates and can access the latest version.

\section{Dataset Structure Explanation}

The dataset used in this research was constructed from two primary sources: RPLAN and ProcTHOR-10k. While Hugging Face hosts a subset version of the dataset containing only ProcTHOR-10k, users must follow the repository's instructions to generate the complete dataset, including RPLAN and ProcTHOR-10k.

The dataset is represented in a JSON format to encapsulate the floorplans' numerical properties and spatial relationships. Each floorplan consists of a series of attributes that define its geometry and metadata. The main fields in the JSON structure include:

\begin{itemize}
\item \textbf{room\_count:} The total number of rooms in the floorplan.
\item  \textbf{total\_area:} The overall area of the floorplan in square units.
\item \textbf{room\_types:} A list of strings indicating the types of rooms present.
\item \textbf{rooms:} A list of dictionaries, each representing an individual room with the following fields:
    \begin{itemize}
    \item \textbf{area:} The area of the room.
    \item \textbf{floor\_polygon:} A list of vertices defining the room's layout, where each vertex has x and y coordinates.
    \item \textbf{is\_regular:} A boolean indicating if the room's shape is rectangular.
    \item \textbf{height:} The y-axis length of the rectangle bounding box enclosing the room
    \item \textbf{width:} The x-axis length of the rectangle bounding box enclosing the room
    \item \textbf{id:} A unique identifier for the room.
    \item \textbf{room\_type:} The type of the room.
    \end{itemize}
\item \textbf{edges:} A list defining the connections between rooms, used for bubble diagram generation.
\end{itemize}

\section{Structured Metadata}
The structured metadata can be found in the \textit{croissant.json} file.

\section{Reproducibility}
Our reported results are reproducible. Code used to train our model, to generate samples, and to evaluate our results are all made publically available at \textbf{https://github.com/plstory/DS2D}

In also includes instructions on how to retrieve datasets, where to put them, and how to download our pre-trained weights. If one would like to train our model from scratch, the repository contains directions on how to do that as well. It also provides step by step instruction on how to generate results and to evaluate them.

%This repository will also be actively maintained and updated for better code-readability and ease-of-use. We will also update instructions in the Readme file accordingly, e.g. when datasets get hosted on a different place for better accessibility. We will continuously update the repository to make sure it is easy to reproduce our results.
